# Supplementary material for: Localized Excitons in Defective Monolayer Germanium Selenide
Source: arXiv:2005.10102 ancillary file (2020-05-20)
Supplement: Supplementary file 1 [file Supplemental_Materials.pdf]

# Supplemental Material: Localized Excitons in Defective Monolayer Germanium Selenide


Arielle Cohen
*Division of Materials Science and Engineering, Boston University, Boston, MA 02215*

D. Kirk Lewis
*Department of Electrical and Computer Engineering, Boston University, Boston, MA 02215*

Tianlun Huang
*Division of Materials Science and Engineering, Boston University, Boston, MA 02215, USA*

Sahar Sharifzadeh
*Department of Electrical and Computer Engineering, Boston University, Boston, MA 02215 and Division of Materials Science and Engineering, Boston University, Boston, MA 02215*


## I. DEFECT STATE IDENTIFICATION

$\epsilon_{d,corr}$ is applied to defect-centered bands identified by their spatial extent. For each band, the spatial extent of the orbital is calculated for the orbital density at the $\Gamma$ point and an average of the orbitals at all k-points. The spatial extent $\langle \mathbf{r} \rangle$ is calculated as

$$\langle \mathbf{r} \rangle = \frac{\int |\mathbf{r} - \mathbf{r_d}| \rho(\mathbf{r}) dr^3}{\int \rho(\mathbf{r}) dr^3}, \tag{1}$$

where $\mathbf{r_d}$ is the center of mass of the electron density.

Table I presents the calculated $\langle \mathbf{r} \rangle$ for near-gap states. The orbitals associated with these states appear in Figure 3 in the main text. The three states identified as defect-centered are labeled as "Defect 1", "Defect 2", and "Defect 3". The pristine-like states (such as the valence band (VB)) have an average extent of $\sim$ 8 Å, at $\mathbf{k} = \Gamma$ and a bandwidth of $\sim$ 0.3 eV. With the introduction of the defect, states identified as defect-like show a reduced extent and a reduced bandwidth. This is best illustrated for Defect 3, with extent of only $\sim$ 4 Å both when only the orbital at $\mathbf{k} = \Gamma$ is considered and when orbitals are averaged over all k-points. Defect 1 and Defect 3 both have very low bandwidths, of less than 0.1 Å. The extent of Defect 1, Defect 2, CB and CB +1 are more ambiguous in that the orbital extent at $\Gamma$ is different than when the orbitals are averaged over all k. We choose the states identified as Defects 1 and 2 due to the localization for the orbital at $\Gamma$.

TABLE I. Calculated orbital spatial extent $\langle \mathbf{r} \rangle$ as defined by Equation 1 for near-gap states

| | VB | Defect 1 | Defect 2 | Defect 3 | CB | CB + 1 |
|---|---|---|---|---|---|---|
| $\mathbf{k} = \Gamma$ (Å) | 8.1 | 5.0 | 7.0 | 4.2 | 8.1 | 8.2 |
| All $\mathbf{k}$ (Å) | 8.3 | 6.8 | 6.5 | 3.9 | 6.1 | 6.8 |
| Bandwidth (eV) | 0.33 | 0.08 | 0.23 | 0.08 | 0.34 | 0.27 |

## II. ELECTRON-HOLE CORRELATION ENVELOPE FUNCTION FOR DELOCALIZED PRISTINE-LIKE TRANSITIONS

Figures 1 and 2 show the ECF (calculated according to Equation 2 in the main text) for the lowest energy Wannier-Mott exciton in the pristine monolayer GeSe and the second excited state for the defective monolayer GeSe, respectively.

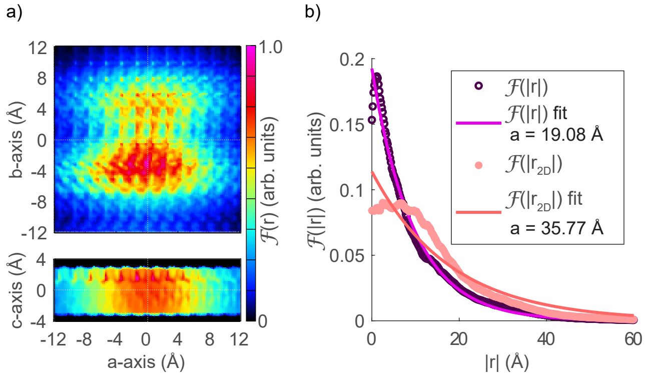


FIG. 1. a) Two-dimensional ECF for pristine monolayer GeSe top view and side view. b) Radial ECF calculated in the a-b plane.

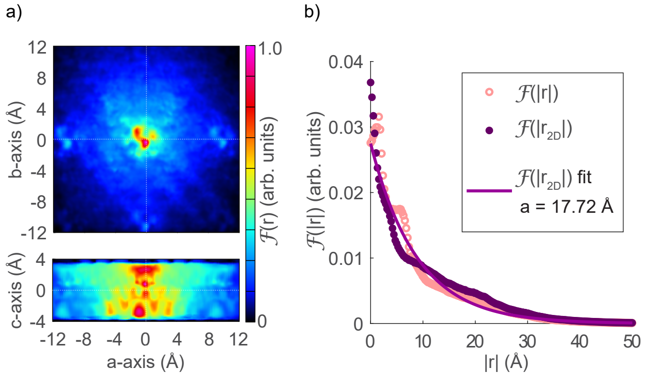


FIG. 2. a) Two-dimensional ECF for the second energy transition in with defect GeSe top view and side view. b) Radial ECF calculated in the a-b plane.
